# Supplementary material for: Fooling Explanations in Text Classifiers
Source: arXiv:2206.03178 source file (2022-06-07)
Supplement: Supplementary file 2 [file robustness_agnews.tex]

\begin{longtable}[c]{ccc}
%		\caption{Further results on the AG's News dataset.\label{apn:additionalresults}}\\	
%		\endhead
		
		\corrlegend
		& \toplegend
		& \evallegend
		
		\endfoot
		
		\endlastfoot

		% AG's News
        \multicolumn{3}{c}{\textbf{CNN - Integrated Gradients (IG) on AG's News}}
\\
        \correlationplot{agnews}{cnn}{IG}
        & \intersectionplot{agnews}{cnn}{IG}
        & \evalplot{agnews}{cnn}{IG}
\\
        \multicolumn{3}{c}{\textbf{LSTM - Saliency Maps (S) on AG's News}}
\\
        \correlationplot{agnews}{lstm}{S}
        & \intersectionplot{agnews}{lstm}{S}
        & \evalplot{agnews}{lstm}{S}
\\
        \multicolumn{3}{c}{\textbf{LSTM - Integrated Gradients (IG) on AG's News}}
\\
        \correlationplot{agnews}{lstm}{IG}
        & \intersectionplot{agnews}{lstm}{IG}
        & \evalplot{agnews}{lstm}{IG}
\\
        \multicolumn{3}{c}{\textbf{LSTMAtt - Saliency Maps (S) on AG's News}}
\\
        \correlationplot{agnews}{lstmatt}{S}
        & \intersectionplot{agnews}{lstmatt}{S}
        & \evalplot{agnews}{lstmatt}{S}
\\
\pagebreak
        \multicolumn{3}{c}{\textbf{LSTMAtt - Integrated Gradients (IG) on AG's News}}
\\
        \correlationplot{agnews}{lstmatt}{IG}
        & \intersectionplot{agnews}{lstmatt}{IG}
        & \evalplot{agnews}{lstmatt}{IG}
\\
        \multicolumn{3}{c}{\textbf{LSTMAtt - Attention (A) on AG's News}}
\\
        \correlationplot{agnews}{lstmatt}{A}
        & \intersectionplot{agnews}{lstmatt}{A}
        & \evalplot{agnews}{lstmatt}{A}
\\
        \multicolumn{3}{c}{\textbf{BERT - Saliency Maps (S) on AG's News}}
\\
        \correlationplot{agnews}{bert}{S}
        & \intersectionplot{agnews}{bert}{S}
        & \evalplot{agnews}{bert}{S}
\\
        \multicolumn{3}{c}{\textbf{BERT - Integrated Gradients (IG) on AG's News}}
\\
        \correlationplot{agnews}{bert}{IG}
        & \intersectionplot{agnews}{bert}{IG}
        & \evalplot{agnews}{bert}{IG}
\\
        \multicolumn{3}{c}{\textbf{BERT - Attention (A) on AG's News}}
\\
        \correlationplot{agnews}{bert}{A}
        & \intersectionplot{agnews}{bert}{A}
        & \evalplot{agnews}{bert}{A}
\\
\pagebreak
        \multicolumn{3}{c}{\textbf{RoBERTa - Saliency Maps (S) on AG's News}}
\\
        \correlationplot{agnews}{roberta}{S}
        & \intersectionplot{agnews}{roberta}{S}
        & \evalplot{agnews}{roberta}{S}
\\
        \multicolumn{3}{c}{\textbf{RoBERTa - Integrated Gradients (IG) on AG's News}}
\\
        \correlationplot{agnews}{roberta}{IG}
        & \intersectionplot{agnews}{roberta}{IG}
        & \evalplot{agnews}{roberta}{IG}
\\
        \multicolumn{3}{c}{\textbf{RoBERTa - Attention (A) on AG's News}}
\\
        \correlationplot{agnews}{roberta}{A}
        & \intersectionplot{agnews}{roberta}{A}
        & \evalplot{agnews}{roberta}{A}
\\
        \multicolumn{3}{c}{\textbf{XLNet - Saliency Maps (S) on AG's News}}
\\
        \correlationplot{agnews}{xlnet}{S}
        & \intersectionplot{agnews}{xlnet}{S}
        & \evalplot{agnews}{xlnet}{S}
\\
        \multicolumn{3}{c}{\textbf{XLNet - Integrated Gradients (IG) on AG's News}}
\\
        \correlationplot{agnews}{xlnet}{IG}
        & \intersectionplot{agnews}{xlnet}{IG}
        & \evalplot{agnews}{xlnet}{IG}
\\
\pagebreak
        \multicolumn{3}{c}{\textbf{XLNet - Attention (A) on AG's News}}
\\
        \correlationplot{agnews}{xlnet}{A}
        & \intersectionplot{agnews}{xlnet}{A}
        & \evalplot{agnews}{xlnet}{A}
\\

\end{longtable}
