# Supplementary material for: Fooling Explanations in Text Classifiers
Source: arXiv:2206.03178 source file (2022-06-07)
Supplement: Supplementary file 3 [file robustness_fakenews.tex]

\begin{longtable}[c]{ccc}
%		\caption{Further results on the AG's News dataset.\label{apn:additionalresults}}\\	
%		\endhead
		
		\corrlegend
		& \toplegend
		& \evallegend
		
		\endfoot
		
		\endlastfoot

% Fake News
        \multicolumn{3}{c}{\textbf{CNN - Saliency Maps (S) on Fake News}}
\\
        \correlationplot{fakenews}{cnn}{S}
        & \intersectionplot{fakenews}{cnn}{S}
        & \evalplot{fakenews}{cnn}{S}
\\
        \multicolumn{3}{c}{\textbf{CNN - Integrated Gradients (IG) on Fake News}}
\\
        \correlationplot{fakenews}{cnn}{IG}
        & \intersectionplot{fakenews}{cnn}{IG}
        & \evalplot{fakenews}{cnn}{IG}
\\
\pagebreak
        \multicolumn{3}{c}{\textbf{LSTM - Saliency Maps (S) on Fake News}}
\\
        \correlationplot{fakenews}{lstm}{S}
        & \intersectionplot{fakenews}{lstm}{S}
        & \evalplot{fakenews}{lstm}{S}
\\
        \multicolumn{3}{c}{\textbf{LSTM - Integrated Gradients (IG) on Fake News}}
\\
        \correlationplot{fakenews}{lstm}{IG}
        & \intersectionplot{fakenews}{lstm}{IG}
        & \evalplot{fakenews}{lstm}{IG}
\\
        \multicolumn{3}{c}{\textbf{LSTMAtt - Saliency Maps (S) on Fake News}}
\\
        \correlationplot{fakenews}{lstmatt}{S}
        & \intersectionplot{fakenews}{lstmatt}{S}
        & \evalplot{fakenews}{lstmatt}{S}
\\
        \multicolumn{3}{c}{\textbf{LSTMAtt - Integrated Gradients (IG) on Fake News}}
\\
        \correlationplot{fakenews}{lstmatt}{IG}
        & \intersectionplot{fakenews}{lstmatt}{IG}
        & \evalplot{fakenews}{lstmatt}{IG}
\\
        \multicolumn{3}{c}{\textbf{LSTMAtt - Attention (A) on Fake News}}
\\
        \correlationplot{fakenews}{lstmatt}{A}
        & \intersectionplot{fakenews}{lstmatt}{A}
        & \evalplot{fakenews}{lstmatt}{A}
\\
\pagebreak
        \multicolumn{3}{c}{\textbf{BERT - Saliency Maps (S) on Fake News}}
\\
        \correlationplot{fakenews}{bert}{S}
        & \intersectionplot{fakenews}{bert}{S}
        & \evalplot{fakenews}{bert}{S}
\\
%        \multicolumn{3}{c}{\textbf{BERT - Integrated Gradients (IG) on Fake News}}
%\\
%        \correlationplot{fakenews}{bert}{IG}
%        & \intersectionplot{fakenews}{bert}{IG}
%        & \evalplot{fakenews}{bert}{IG}
%\\
%        \multicolumn{3}{c}{\textbf{BERT - Attention (A) on Fake News}}
%\\
%        \correlationplot{fakenews}{bert}{A}
%        & \intersectionplot{fakenews}{bert}{A}
%        & \evalplot{fakenews}{bert}{A}
%\\
        \multicolumn{3}{c}{\textbf{RoBERTa - Saliency Maps (S) on Fake News}}
\\
        \correlationplot{fakenews}{roberta}{S}
        & \intersectionplot{fakenews}{roberta}{S}
        & \evalplot{fakenews}{roberta}{S}
\\
        \multicolumn{3}{c}{\textbf{RoBERTa - Attention (A) on Fake News}}
\\
        \correlationplot{fakenews}{roberta}{A}
        & \intersectionplot{fakenews}{roberta}{A}
        & \evalplot{fakenews}{roberta}{A}
\\
        \multicolumn{3}{c}{\textbf{XLNet - Saliency Maps (S) on Fake News}}
\\
        \correlationplot{fakenews}{xlnet}{S}
        & \intersectionplot{fakenews}{xlnet}{S}
        & \evalplot{fakenews}{xlnet}{S}
\\
        \multicolumn{3}{c}{\textbf{XLNet - Integrated Gradients (IG) on Fake News}}
\\
        \correlationplot{fakenews}{xlnet}{IG}
        & \intersectionplot{fakenews}{xlnet}{IG}
        & \evalplot{fakenews}{xlnet}{IG}

\end{longtable}
