# Supplementary material for: Fooling Explanations in Text Classifiers
Source: arXiv:2206.03178 source file (2022-06-07)
Supplement: Supplementary file 4 [file robustness_imdb.tex]

\begin{longtable}[c]{ccc}
%		\caption{Further results on the AG's News dataset.\label{apn:additionalresults}}\\	
%		\endhead
		
		\corrlegend
		& \toplegend
		& \evallegend
		
		\endfoot
		
		\endlastfoot

% IMDB
        \multicolumn{3}{c}{\textbf{CNN - Saliency Maps (S) on IMDB}}
\\
        \correlationplot{imdb}{cnn}{S}
        & \intersectionplot{imdb}{cnn}{S}
        & \evalplot{imdb}{cnn}{S}
\\
        \multicolumn{3}{c}{\textbf{CNN - Integrated Gradients (IG) on IMDB}}
\\
        \correlationplot{imdb}{cnn}{IG}
        & \intersectionplot{imdb}{cnn}{IG}
        & \evalplot{imdb}{cnn}{IG}
\\
        \multicolumn{3}{c}{\textbf{LSTM - Saliency Maps (S) on IMDB}}
\\
        \correlationplot{imdb}{lstm}{S}
        & \intersectionplot{imdb}{lstm}{S}
        & \evalplot{imdb}{lstm}{S}
\\
        \multicolumn{3}{c}{\textbf{LSTM - Integrated Gradients (IG) on IMDB}}
\\
        \correlationplot{imdb}{lstm}{IG}
        & \intersectionplot{imdb}{lstm}{IG}
        & \evalplot{imdb}{lstm}{IG}
\\
\pagebreak
        \multicolumn{3}{c}{\textbf{LSTMAtt - Saliency Maps (S) on IMDB}}
\\
        \correlationplot{imdb}{lstmatt}{S}
        & \intersectionplot{imdb}{lstmatt}{S}
        & \evalplot{imdb}{lstmatt}{S}
\\
        \multicolumn{3}{c}{\textbf{LSTMAtt - Integrated Gradients (IG) on IMDB}}
\\
        \correlationplot{imdb}{lstmatt}{IG}
        & \intersectionplot{imdb}{lstmatt}{IG}
        & \evalplot{imdb}{lstmatt}{IG}
\\
        \multicolumn{3}{c}{\textbf{BERT - Saliency Maps (S) on IMDB}}
\\
        \correlationplot{imdb}{bert}{S}
        & \intersectionplot{imdb}{bert}{S}
        & \evalplot{imdb}{bert}{S}
\\
        \multicolumn{3}{c}{\textbf{BERT - Integrated Gradients (IG) on IMDB}}
\\
        \correlationplot{imdb}{bert}{IG}
        & \intersectionplot{imdb}{bert}{IG}
        & \evalplot{imdb}{bert}{IG}
\\
        \multicolumn{3}{c}{\textbf{BERT - Attention (A) on IMDB}}
\\
        \correlationplot{imdb}{bert}{A}
        & \intersectionplot{imdb}{bert}{A}
        & \evalplot{imdb}{bert}{A}
\\
\pagebreak
        \multicolumn{3}{c}{\textbf{RoBERTa - Saliency Maps (S) on IMDB}}
\\
        \correlationplot{imdb}{roberta}{S}
        & \intersectionplot{imdb}{roberta}{S}
        & \evalplot{imdb}{roberta}{S}
\\
        \multicolumn{3}{c}{\textbf{RoBERTa - Integrated Gradients (IG) on IMDB}}
\\
        \correlationplot{imdb}{roberta}{IG}
        & \intersectionplot{imdb}{roberta}{IG}
        & \evalplot{imdb}{roberta}{IG}
\\
        \multicolumn{3}{c}{\textbf{RoBERTa - Attention (A) on IMDB}}
\\
        \correlationplot{imdb}{roberta}{A}
        & \intersectionplot{imdb}{roberta}{A}
        & \evalplot{imdb}{roberta}{A}
\\
        \multicolumn{3}{c}{\textbf{XLNet - Saliency Maps (S) on IMDB}}
\\
        \correlationplot{imdb}{xlnet}{S}
        & \intersectionplot{imdb}{xlnet}{S}
        & \evalplot{imdb}{xlnet}{S}
\\
        \multicolumn{3}{c}{\textbf{XLNet - Integrated Gradients (IG) on IMDB}}
\\
        \correlationplot{imdb}{xlnet}{IG}
        & \intersectionplot{imdb}{xlnet}{IG}
        & \evalplot{imdb}{xlnet}{IG}
\\
\pagebreak
        \multicolumn{3}{c}{\textbf{XLNet - Attention (A) on IMDB}}
\\
        \correlationplot{imdb}{xlnet}{A}
        & \intersectionplot{imdb}{xlnet}{A}
        & \evalplot{imdb}{xlnet}{A}
%\\

\end{longtable}
