# Supplementary material for: Fooling Explanations in Text Classifiers
Source: arXiv:2206.03178 source file (2022-06-07)
Supplement: Supplementary file 5 [file robustness_mr.tex]

\begin{longtable}[c]{ccc}
%		\caption{Further results on the AG's News dataset.\label{apn:additionalresults}}\\	
%		\endhead
		
		\corrlegend
		& \toplegend
		& \evallegend
		
		\endfoot
		
		\endlastfoot
		
% MR
        \multicolumn{3}{c}{\textbf{CNN - Saliency Maps (S) on MR}}
\\
        \correlationplot{mr}{cnn}{S}
        & \intersectionplot{mr}{cnn}{S}
        & \evalplot{mr}{cnn}{S}
\\
        \multicolumn{3}{c}{\textbf{CNN - Integrated Gradients (IG) on MR}}
\\
        \correlationplot{mr}{cnn}{IG}
        & \intersectionplot{mr}{cnn}{IG}
        & \evalplot{mr}{cnn}{IG}
\\
        \multicolumn{3}{c}{\textbf{LSTM - Saliency Maps (S) on MR}}
\\
        \correlationplot{mr}{lstm}{S}
        & \intersectionplot{mr}{lstm}{S}
        & \evalplot{mr}{lstm}{S}
\\
        \multicolumn{3}{c}{\textbf{LSTM - Integrated Gradients (IG) on MR}}
\\
        \correlationplot{mr}{lstm}{IG}
        & \intersectionplot{mr}{lstm}{IG}
        & \evalplot{mr}{lstm}{IG}
\\
\pagebreak
        \multicolumn{3}{c}{\textbf{LSTMAtt - Saliency Maps (S) on MR}}
\\
        \correlationplot{mr}{lstmatt}{S}
        & \intersectionplot{mr}{lstmatt}{S}
        & \evalplot{mr}{lstmatt}{S}
\\
        \multicolumn{3}{c}{\textbf{LSTMAtt - Integrated Gradients (IG) on MR}}
\\
        \correlationplot{mr}{lstmatt}{IG}
        & \intersectionplot{mr}{lstmatt}{IG}
        & \evalplot{mr}{lstmatt}{IG}
\\
        \multicolumn{3}{c}{\textbf{LSTMAtt - Attention (A) on MR}}
\\
        \correlationplot{mr}{lstmatt}{A}
        & \intersectionplot{mr}{lstmatt}{A}
        & \evalplot{mr}{lstmatt}{A}
\\
        \multicolumn{3}{c}{\textbf{BERT - Saliency Maps (S) on MR}}
\\
        \correlationplot{mr}{bert}{S}
        & \intersectionplot{mr}{bert}{S}
        & \evalplot{mr}{bert}{S}
\\
        \multicolumn{3}{c}{\textbf{BERT - Integrated Gradients (IG) on MR}}
\\
        \correlationplot{mr}{bert}{IG}
        & \intersectionplot{mr}{bert}{IG}
        & \evalplot{mr}{bert}{IG}
\\
\pagebreak
        \multicolumn{3}{c}{\textbf{BERT - Attention (A) on MR}}
\\
        \correlationplot{mr}{bert}{A}
        & \intersectionplot{mr}{bert}{A}
        & \evalplot{mr}{bert}{A}
\\
        \multicolumn{3}{c}{\textbf{RoBERTa - Integrated Gradients (IG) on MR}}
\\
        \correlationplot{mr}{roberta}{IG}
        & \intersectionplot{mr}{roberta}{IG}
        & \evalplot{mr}{roberta}{IG}
\\
        \multicolumn{3}{c}{\textbf{RoBERTa - Attention (A) on MR}}
\\
        \correlationplot{mr}{roberta}{A}
        & \intersectionplot{mr}{roberta}{A}
        & \evalplot{mr}{roberta}{A}
\\
        \multicolumn{3}{c}{\textbf{XLNet - Saliency Maps (S) on MR}}
\\
        \correlationplot{mr}{xlnet}{S}
        & \intersectionplot{mr}{xlnet}{S}
        & \evalplot{mr}{xlnet}{S}
\\
        \multicolumn{3}{c}{\textbf{XLNet - Integrated Gradients (IG) on MR}}
\\
        \correlationplot{mr}{xlnet}{IG}
        & \intersectionplot{mr}{xlnet}{IG}
        & \evalplot{mr}{xlnet}{IG}
\\
\pagebreak
        \multicolumn{3}{c}{\textbf{XLNet - Attention (A) on MR}}
\\
        \correlationplot{mr}{xlnet}{A}
        & \intersectionplot{mr}{xlnet}{A}
        & \evalplot{mr}{xlnet}{A}
 	
\end{longtable}
