# Supplementary material for: Fooling Explanations in Text Classifiers
Source: arXiv:2206.03178 source file (2022-06-07)
Supplement: Supplementary file 6 [file robustness_yelp.tex]

\begin{longtable}[c]{ccc}
%		\caption{Further results on the AG's News dataset.\label{apn:additionalresults}}\\	
%		\endhead
		
		\corrlegend
		& \toplegend
		& \evallegend
		
		\endfoot
		
		\endlastfoot

% Yelp
        \multicolumn{3}{c}{\textbf{CNN - Saliency Maps (S) on Yelp}}
\\
        \correlationplot{yelp}{cnn}{S}
        & \intersectionplot{yelp}{cnn}{S}
        & \evalplot{yelp}{cnn}{S}
\\
        \multicolumn{3}{c}{\textbf{CNN - Integrated Gradients (IG) on Yelp}}
\\
        \correlationplot{yelp}{cnn}{IG}
        & \intersectionplot{yelp}{cnn}{IG}
        & \evalplot{yelp}{cnn}{IG}
\\
        \multicolumn{3}{c}{\textbf{LSTM - Saliency Maps (S) on Yelp}}
\\
        \correlationplot{yelp}{lstm}{S}
        & \intersectionplot{yelp}{lstm}{S}
        & \evalplot{yelp}{lstm}{S}
\\
        \multicolumn{3}{c}{\textbf{LSTM - Integrated Gradients (IG) on Yelp}}
\\
        \correlationplot{yelp}{lstm}{IG}
        & \intersectionplot{yelp}{lstm}{IG}
        & \evalplot{yelp}{lstm}{IG}
\\
\pagebreak
        \multicolumn{3}{c}{\textbf{LSTMAtt - Saliency Maps (S) on Yelp}}
\\
        \correlationplot{yelp}{lstmatt}{S}
        & \intersectionplot{yelp}{lstmatt}{S}
        & \evalplot{yelp}{lstmatt}{S}
\\
        \multicolumn{3}{c}{\textbf{LSTMAtt - Integrated Gradients (IG) on Yelp}}
\\
        \correlationplot{yelp}{lstmatt}{IG}
        & \intersectionplot{yelp}{lstmatt}{IG}
        & \evalplot{yelp}{lstmatt}{IG}
\\
        \multicolumn{3}{c}{\textbf{LSTMAtt - Attention (A) on Yelp}}
\\
        \correlationplot{yelp}{lstmatt}{A}
        & \intersectionplot{yelp}{lstmatt}{A}
        & \evalplot{yelp}{lstmatt}{A}
\\
        \multicolumn{3}{c}{\textbf{BERT - Saliency Maps (S) on Yelp}}
\\
        \correlationplot{yelp}{bert}{S}
        & \intersectionplot{yelp}{bert}{S}
        & \evalplot{yelp}{bert}{S}
\\
        \multicolumn{3}{c}{\textbf{BERT - Attention (A) on Yelp}}
\\
        \correlationplot{yelp}{bert}{A}
        & \intersectionplot{yelp}{bert}{A}
        & \evalplot{yelp}{bert}{A}
\\
\pagebreak
        \multicolumn{3}{c}{\textbf{RoBERTa - Saliency Maps (S) on Yelp}}
\\
        \correlationplot{yelp}{roberta}{S}
        & \intersectionplot{yelp}{roberta}{S}
        & \evalplot{yelp}{roberta}{S}
\\
        \multicolumn{3}{c}{\textbf{RoBERTa - Integrated Gradients (IG) on Yelp}}
\\
        \correlationplot{yelp}{roberta}{IG}
        & \intersectionplot{yelp}{roberta}{IG}
        & \evalplot{yelp}{roberta}{IG}
\\
        \multicolumn{3}{c}{\textbf{RoBERTa - Attention (A) on Yelp}}
\\
        \correlationplot{yelp}{roberta}{A}
        & \intersectionplot{yelp}{roberta}{A}
        & \evalplot{yelp}{roberta}{A}
% \\
%         \multicolumn{3}{c}{\textbf{XLNet - Saliency Maps (S) on Yelp}}
% \\
%         \correlationplot{yelp}{xlnet}{S}
%         & \intersectionplot{yelp}{xlnet}{S}
%         & \evalplot{yelp}{xlnet}{S}
% \\
%         \multicolumn{3}{c}{\textbf{XLNet - Integrated Gradients (IG) on Yelp}}
% \\
%         \correlationplot{yelp}{xlnet}{IG}
%         & \intersectionplot{yelp}{xlnet}{IG}
%         & \evalplot{yelp}{xlnet}{IG}
% \\
%         \multicolumn{3}{c}{\textbf{XLNet - Attention (A) on Yelp}}
% \\
%         \correlationplot{yelp}{xlnet}{A}
%         & \intersectionplot{yelp}{xlnet}{A}
%         & \evalplot{yelp}{xlnet}{A}
\end{longtable}
