# Supplementary material for: Fooling Explanations in Text Classifiers
Source: arXiv:2206.03178 source file (2022-06-07)
Supplement: Supplementary file 7 [file tef_operation_example.tex]

Given classifier $F$, input sample $s\;\mathrm{=}$ \textit{"a poignant comedy that offers food for thought ."}, original attribution scores $A(s, F, l)$, 
find the adversarial sequence of tokens $\mathrm{s_{adv}}$ that minimizes $\mathrm{PCC}\,[A(s, F, l), \;A(s_{adv}, F, l)]$ such that at most $\rho_{max} = 25\%$ of words are changed, $\argmax_{l}F(s, l) = \argmax_{l}F(s_{adv}, l) = \mathrm{\mathbf{Pos.}}$ and $s_{adv}$ fulfills the locality constraints described in Section \ref{sec:methods}, namely each replacement is a synonym of the original word \citep{counterfitted}, the replacement word needs to have the same Part Of Speech computed by SpaCy \citep{spacy} and stop words can not be replaced.

\addtolength{\tabcolsep}{-3pt}  % Default is 6pt 
\begin{table}[H]
    \centering
    \begin{tabular}{c|ccccccccc}
         $w_i$&0&1&2&3&4&5&6&7&8\\
         \hline
         $s$    & \textcolor[rgb]{0,0,0}{a}   & \textcolor[rgb]{0,0,0.08}{poignant}    & \textcolor[rgb]{0.4,0,0}{\textbf{comedy}}  & \textcolor[rgb]{0.05,0,0}{that}    & \textcolor[rgb]{0.16,0,0}{\textbf{offers}}   & \textcolor[rgb]{0.23,0,0}{\textbf{food}}    & \textcolor[rgb]{0.03,0,0}{for} & \textcolor[rgb]{0.22,0,0}{\textbf{thought}} & \textcolor[rgb]{0,0,0}{.}\\
         $A(s)$ & 0.0       & -0.08         &  0.4          &  0.05     &  0.16         &  0.23     &  0.03     &  0.22     & 0.0\\
    \end{tabular}
    % \caption{Caption}
    % \label{tab:my_label}
\end{table}

The word importance ranking from Section \ref{sec:methods} yields \textit{poignant} and \textit{comedy} (in this order) to be the $\lfloor 9 \cdot 0.25 \rfloor = 2$ most important tokens, therefore the candidate replacements for only those are considered. This results in the following two steps of TEF.\\%
\paragraph{1. Step.} Replace the most important word \textit{poignant} with it's best candidate, measured by lowest PCC. This candidate is the word \textit{distressing}.
\begin{table}[H]
    \centering
    \begin{tabular}{c|ccccccccc|c}
         $w_i$&0&1&2&3&4&5&6&7&8&PCC\\
         \hline
         %  0.01 -0.21 0.45 0.05 0.18 0.25 0.04 0.22 0.01
         $s'$    & \textcolor[rgb]{0.01,0,0}{a}   & \cellcolor{yellow!25}\textcolor[rgb]{0,0,0.21}{heartbreaking}    & \textcolor[rgb]{0.45,0,0}{comedy}  & \textcolor[rgb]{0.05,0,0}{that}    & \textcolor[rgb]{0.18,0,0}{offers}   & \textcolor[rgb]{0.25,0,0}{food}    & \textcolor[rgb]{0.04,0,0}{for} & \textcolor[rgb]{0.22,0,0}{thought} & \textcolor[rgb]{0.01,0,0}{.}&\\
         $A(s')$ & 0.01      & -0.21         &  0.45          &  0.05     &  0.18         &  0.25     &  0.04     &  0.22     & 0.01 & 0.98\\
         
         \hline
         % -0.13 0.15 1.18 0.12 -1.4 0.75 -0.14 0.37 0.09
         $s'$    & \textcolor[rgb]{0,0,0.013}{a}   & \cellcolor{yellow!25}\textcolor[rgb]{0.15,0,0}{distressing}    & \textcolor[rgb]{1,0,0}{comedy}  & \textcolor[rgb]{0.12,0,0}{that}    & \textcolor[rgb]{0,0,1}{offers}   & \textcolor[rgb]{0.75,0,0}{food}    & \textcolor[rgb]{0,0,0.14}{for} & \textcolor[rgb]{0.37,0,0}{thought} & \textcolor[rgb]{0.09,0,0}{.}&\\
         $A(s')$ & -0.13       & 0.15         &  1.18          &  0.12     &  -1.4         &  0.75     &  -0.14    &  0.37     & 0.09 & \textbf{0.44}\\
         
         \hline
         $s'$    & \textcolor[rgb]{0,0,0}{a}   & \cellcolor{yellow!25}\textcolor[rgb]{0,0,0}{alarm}    & \textcolor[rgb]{0,0,0}{comedy}  & \textcolor[rgb]{0,0,0}{that}    & \textcolor[rgb]{0,0,0}{offers}   & \textcolor[rgb]{0,0,0}{food}    & \textcolor[rgb]{0,0,0}{for} & \textcolor[rgb]{0,0,0}{thought} & \textcolor[rgb]{0,0,0}{.}&\\
         $A(s')$ & \multicolumn{9}{c|}{\textcolor[rgb]{1,0,0}{Failed POS-Filter}} & -\\
         
         \hline
         $s'$    & \textcolor[rgb]{0,0,0}{a}   & \cellcolor{yellow!25}\textcolor[rgb]{0,0,0}{agonizing}    & \textcolor[rgb]{0,0,0}{comedy}  & \textcolor[rgb]{0,0,0}{that}    & \textcolor[rgb]{0,0,0}{offers}   & \textcolor[rgb]{0,0,0}{food}    & \textcolor[rgb]{0,0,0}{for} & \textcolor[rgb]{0,0,0}{thought} & \textcolor[rgb]{0,0,0}{.}&\\
         $A(s')$ & \multicolumn{9}{c|}{\textcolor[rgb]{1,0,0}{Failed Prediction-Filter}} & -\\
         
     \end{tabular}
    % \caption{Caption}
    % \label{tab:my_label}
\end{table}%
\paragraph{2. Step.} Replace the second-most important word \textit{comedy} with the best valid candidate, in this case the token \textit{comic}.%
\begin{table}[H]
    \centering
    \begin{tabular}{c|ccccccccc|c}
         $w_i$&0&1&2&3&4&5&6&7&8&PCC\\
         \hline
    
         % -0.09 0.01 0.34 0.27 0.20 -0.02 0.02 0.27 0.05
         $s'$    & \textcolor[rgb]{0,0,0.09}{a}   & \textcolor[rgb]{0.01,0,0}{distressing}    & \cellcolor{yellow!25}\textcolor[rgb]{0.34,0,0}{\textbf{humor}}  & \textcolor[rgb]{0.27,0,0}{\textbf{that}}    & \textcolor[rgb]{0.2,0,0}{\textbf{offers}}   & \textcolor[rgb]{0,0,0.02}{food}    & \textcolor[rgb]{0.02,0,0}{for} & \textcolor[rgb]{0.27,0,0}{\textbf{thought}} & \textcolor[rgb]{0.05,0,0}{.}&\\
         $A(s')$ & -0.09       & 0.01         &  0.34          &  0.27     &  0.2         &  -0.02     &  0.02     &  0.27     & 0.05 & 0.63\\
         
         \hline
         % -0.02 0.04 0.05 0.02 0.57 -0.13 0.01 0.46 0.04
         $s'$    & \textcolor[rgb]{0,0,0.02}{a}   & \textcolor[rgb]{0.04,0,0}{distressing}    & \cellcolor{yellow!25}\textcolor[rgb]{0.05,0,0}{comic}  & \textcolor[rgb]{0.20,0,0}{\textbf{that}}    & \textcolor[rgb]{0.57,0,0}{\textbf{offers}}   & \textcolor[rgb]{0,0,0.013}{food}    & \textcolor[rgb]{0.01,0,0}{for} & \textcolor[rgb]{0.46,0,0}{thought} & \textcolor[rgb]{0.04,0,0}{.}&\\
         $A(s')$ & -0.02       & 0.04         &  0.05          &  0.02     &  0.57         &  -0.13     &  0.01     &  0.46     & 0.04 & \textbf{0.22}\\
         
         \hline
         $s'$    & \textcolor[rgb]{0,0,0}{a}   & \textcolor[rgb]{0,0,0}{distressing}    & \cellcolor{yellow!25}\textcolor[rgb]{0,0,0}{travesty}  & \textcolor[rgb]{0,0,0}{that}    & \textcolor[rgb]{0,0,0}{offers}   & \textcolor[rgb]{0,0,0}{food}    & \textcolor[rgb]{0,0,0}{for} & \textcolor[rgb]{0,0,0}{thought} & \textcolor[rgb]{0,0,0}{.}&\\
         $A(s')$ & \multicolumn{9}{c|}{\textcolor[rgb]{1,0,0}{Failed Prediction-Filter}} & -\\
         
         \hline
         $s'$    & \textcolor[rgb]{0,0,0}{a}   & \textcolor[rgb]{0,0,0}{distressing}    & \cellcolor{yellow!25}\textcolor[rgb]{0,0,0}{humorous}  & \textcolor[rgb]{0,0,0}{that}    & \textcolor[rgb]{0,0,0}{offers}   & \textcolor[rgb]{0,0,0}{food}    & \textcolor[rgb]{0,0,0}{for} & \textcolor[rgb]{0,0,0}{thought} & \textcolor[rgb]{0,0,0}{.}&\\
         $A(s')$ & \multicolumn{9}{c|}{\textcolor[rgb]{1,0,0}{Failed POS-Filter}} & -
    \end{tabular}
    % \caption{Caption}
    % \label{tab:my_label}
\end{table}%
The \textbf{final adversarial sequence} $s_{adv}$ becomes the valid $s'$ with the lowest PCC value, which is given in the following table.%
\begin{table}[H]
    \centering
    \begin{tabular}{c|ccccccccc|c}
         $w_i$&0&1&2&3&4&5&6&7&8&PCC\\
         \hline
         $s$    & \textcolor[rgb]{0,0,0}{a}   & \textcolor[rgb]{0,0,0.08}{poignant}    & \textcolor[rgb]{0.4,0,0}{\textbf{comedy}}  & \textcolor[rgb]{0.05,0,0}{that}    & \textcolor[rgb]{0.16,0,0}{\textbf{offers}}   & \textcolor[rgb]{0.23,0,0}{\textbf{food}}    & \textcolor[rgb]{0.03,0,0}{for} & \textcolor[rgb]{0.22,0,0}{\textbf{thought}} & \textcolor[rgb]{0,0,0}{.}&\\
         $A(s)$ & 0.0       & -0.08         &  0.4          &  0.05     &  0.16         &  0.23     &  0.03     &  0.22     & 0.0 & -\\
         \hline
         $\mathbf{\mathrm{s_{adv}}}$ & \textcolor[rgb]{0,0,0.02}{a}   & \cellcolor{yellow!25}\textcolor[rgb]{0.04,0,0}{distressing}    & \cellcolor{yellow!25}\textcolor[rgb]{0.05,0,0}{comic}  & \textcolor[rgb]{0.20,0,0}{\textbf{that}}    & \textcolor[rgb]{0.57,0,0}{\textbf{offers}}   & \textcolor[rgb]{0,0,0.013}{food}    & \textcolor[rgb]{0.01,0,0}{for} & \textcolor[rgb]{0.46,0,0}{\textbf{thought}} & \textcolor[rgb]{0.04,0,0}{.}&\\
         A($\mathbf{\mathrm{s_{adv}}}$) & -0.02       & 0.04         &  0.05          &  0.02     &  0.57         &  -0.13     &  0.01     &  046     & 0.04 & \textbf{0.22}\\
        
    \end{tabular}
\end{table}
\addtolength{\tabcolsep}{3pt}  % Default is 6pt
